# Supplementary material for: Unveiling diverse nature of core collapse supernovae
Source: arXiv:2312.16266 source file (2023-12-26)
Supplement: Supplementary file 1 [file supplementary_material.pdf]

## APPENDIX A: LOG OF SPECTROSCOPIC AND PHOTOMETRIC OBSERVATIONS

This paper has been typeset from a  $\text{\TeX}/\text{\LaTeX}$  file prepared by the author.

**Table A1.** Spectroscopic observations of SN 2016bau.

Note: All spectra were taken with the Kast spectrograph on the 3.0 m Shane telescope at Lick Observatory.

| UT Date    | MJD       |
|------------|-----------|
| 2016/03/16 | 57463.719 |
| 2016/03/19 | 57466.919 |
| 2016/04/03 | 57481.671 |
| 2016/04/17 | 57495.902 |
| 2016/05/02 | 57510.671 |
| 2016/05/16 | 57524.860 |
| 2016/05/30 | 57538.741 |
| 2016/07/15 | 57584.710 |

**Table A2.** Photometry of SN 2015ap.

| MJD        | <i>B</i><br>(mag) | <i>V</i><br>(mag) | <i>R</i><br>(mag) | <i>I</i><br>(mag) | Telescope<br>(mag) |
|------------|-------------------|-------------------|-------------------|-------------------|--------------------|
| 57274.4258 | 17.35 ± 0.09      | 17.28 ± 0.07      | 17.07 ± 0.05      | 16.75 ± 0.06      | KAIT               |
| 57275.3867 | 16.94 ± 0.09      | 16.83 ± 0.06      | 16.67 ± 0.05      | 16.39 ± 0.06      | KAIT               |
| 57276.3516 | 16.40 ± 0.17      | 16.40 ± 0.11      | 16.39 ± 0.08      | 16.05 ± 0.07      | KAIT               |
| 57279.4336 | 15.79 ± 0.11      | 15.84 ± 0.06      | 15.64 ± 0.05      | 15.39 ± 0.05      | KAIT               |
| 57283.4375 | 15.44 ± 0.01      | 15.26 ± 0.01      | 15.14 ± 0.01      | 14.93 ± 0.01      | Nickel             |
| 57285.5078 | 15.64 ± 0.08      | 15.44 ± 0.04      | 15.20 ± 0.03      | 14.90 ± 0.03      | KAIT               |
| 57286.4062 | 15.70 ± 0.04      | 15.48 ± 0.03      | 15.14 ± 0.02      | 14.87 ± 0.02      | KAIT               |
| 57287.4375 | 15.91 ± 0.05      | 15.47 ± 0.03      | 15.18 ± 0.03      | 14.87 ± 0.03      | KAIT               |
| 57288.4102 | 15.89 ± 0.05      | 15.51 ± 0.03      | 15.17 ± 0.03      | 14.86 ± 0.03      | KAIT               |
| 57290.3555 | 16.07 ± 0.07      | 15.55 ± 0.05      | 15.20 ± 0.03      | 14.87 ± 0.03      | KAIT               |
| 57291.3594 | 16.30 ± 0.09      | 15.58 ± 0.04      | 15.19 ± 0.03      | 14.88 ± 0.013     | KAIT               |
| 57297.4023 | 17.06 ± 0.20      | 16.27 ± 0.07      | 15.71 ± 0.04      | 15.19 ± 0.04      | KAIT               |
| 57298.3906 | 17.30 ± 0.12      | 16.20 ± 0.04      | 15.75 ± 0.03      | 15.23 ± 0.03      | KAIT               |
| 57299.5039 | 17.35 ± 0.15      | 16.53 ± 0.05      | 15.91 ± 0.03      | 15.22 ± 0.03      | KAIT               |
| 57301.4258 | 17.52 ± 0.11      | 16.48 ± 0.04      | 15.98 ± 0.03      | 15.35 ± 0.03      | KAIT               |
| 57302.3125 | 17.43 ± 0.01      | 16.37 ± 0.01      | 15.86 ± 0.01      | 15.33 ± 0.01      | Nickel             |
| 57302.3672 | 17.47 ± 0.08      | 16.52 ± 0.04      | 16.05 ± 0.03      | 15.46 ± 0.03      | KAIT               |
| 57304.4727 | 17.68 ± 0.12      | 16.76 ± 0.07      | 16.19 ± 0.04      | 15.57 ± 0.03      | KAIT               |
| 57305.3828 | 17.90 ± 0.12      | 16.76 ± 0.05      | 16.27 ± 0.03      | 15.61 ± 0.03      | KAIT               |
| 57306.3516 | 17.88 ± 0.18      | 16.84 ± 0.06      | 16.26 ± 0.04      | 15.65 ± 0.04      | KAIT               |
| 57307.3438 | 17.74 ± 0.01      | 16.72 ± 0.01      | 16.18 ± 0.01      | 15.63 ± 0.01      | Nickel             |
| 57307.3945 | 17.82 ± 0.13      | 16.86 ± 0.04      | 16.27 ± 0.03      | 15.76 ± 0.04      | KAIT               |
| 57308.3633 | 17.82 ± 0.12      | 16.83 ± 0.05      | 16.34 ± 0.03      | 15.75 ± 0.04      | KAIT               |
| 57309.4609 | 17.91 ± 0.16      | 16.89 ± 0.08      | 16.35 ± 0.04      | 15.73 ± 0.04      | KAIT               |
| 57317.3047 | 17.98 ± 0.02      | 17.10 ± 0.01      | 16.64 ± 0.01      | 15.99 ± 0.01      | Nickel             |
| 57317.4492 | 18.31 ± 0.24      | 17.25 ± 0.08      | 16.75 ± 0.05      | 16.02 ± 0.04      | KAIT               |
| 57318.3008 | 18.19 ± 0.27      | 17.30 ± 0.09      | 16.72 ± 0.05      | 16.12 ± 0.05      | KAIT               |
| 57319.3984 | 18.22 ± 0.20      | 17.48 ± 0.12      | 16.80 ± 0.05      | 16.12 ± 0.07      | KAIT               |
| 57325.4297 | 18.25 ± 0.38      | 17.14 ± 0.14      | 17.15 ± 0.09      | 16.19 ± 0.07      | KAIT               |
| 57326.3594 | 18.42 ± 0.29      | 17.43 ± 0.07      | 17.03 ± 0.05      | 16.35 ± 0.04      | KAIT               |
| 57327.4297 | 17.98 ± 0.26      | 17.40 ± 0.12      | -                 | -                 | KAIT               |
| 57330.3906 | 18.37 ± 0.22      | 17.58 ± 0.08      | 17.20 ± 0.06      | 16.46 ± 0.05      | KAIT               |
| 57331.3359 | 18.63 ± 0.22      | 17.72 ± 0.08      | 17.16 ± 0.04      | 16.59 ± 0.05      | KAIT               |
| 57332.3047 | 18.21 ± 0.01      | 17.47 ± 0.01      | 17.11 ± 0.01      | 16.47 ± 0.01      | Nickel             |
| 57332.3555 | 18.31 ± 0.18      | 17.57 ± 0.07      | 17.21 ± 0.04      | 16.56 ± 0.04      | KAIT               |
| 57333.3477 | 18.19 ± 0.17      | 17.73 ± 0.09      | 17.23 ± 0.06      | 16.56 ± 0.05      | KAIT               |
| 57334.3789 | 18.35 ± 0.16      | 17.66 ± 0.08      | 17.25 ± 0.06      | 16.51 ± 0.05      | KAIT               |
| 57337.3281 | 18.33 ± 0.20      | 18.01 ± 0.18      | 17.33 ± 0.05      | 16.85 ± 0.06      | KAIT               |
| 57338.2852 | 18.62 ± 0.28      | 17.79 ± 0.12      | 17.30 ± 0.05      | 16.73 ± 0.05      | KAIT               |
| 57339.3125 | 18.45 ± 0.22      | 17.83 ± 0.08      | 17.46 ± 0.05      | 16.75 ± 0.06      | KAIT               |
| 57339.3438 | 18.28 ± 0.02      | 17.64 ± 0.01      | 17.27 ± 0.02      | 16.66 ± 0.01      | Nickel             |
| 57340.3594 | 18.52 ± 0.18      | 17.76 ± 0.07      | 17.40 ± 0.06      | 16.73 ± 0.06      | KAIT               |
| 57343.3906 | 18.31 ± 0.02      | 17.66 ± 0.01      | 17.38 ± 0.02      | 16.64 ± 0.01      | Nickel             |
| 57347.3164 | 18.51 ± 0.03      | 17.73 ± 0.01      | 17.51 ± 0.02      | 17.02 ± 0.02      | Nickel             |
| 57361.2656 | 18.55 ± 0.02      | 18.14 ± 0.01      | 17.93 ± 0.02      | 17.19 ± 0.01      | Nickel             |
| 57425.1641 | 19.22 ± 0.06      | 19.63 ± 0.07      | -                 | -                 | Nickel             |
| 57431.1250 | 19.51 ± 0.10      | 19.48 ± 0.10      | 19.05 ± 0.34      | -                 | Nickel             |
| 57444.1328 | 19.67 ± 0.09      | 20.06 ± 0.10      | 19.82 ± 0.09      | 18.93 ± 0.06      | Nickel             |

**Table A3.** Log of *HST* observations of SN 2015ap.

Note: All exposures were 710 s and there were no detections.

| UT Date    | Filter |
|------------|--------|
| 2017/08/16 | F555W  |
| 2017/02/19 | F814W  |
| 2016/04/03 | F555W  |
| 2016/04/17 | F814W  |

Table A4. Photometry of SN 2016bau

| MJD       | <i>B</i><br>(mag) | <i>V</i><br>(mag) | <i>R</i><br>(mag) | <i>clear</i><br>(mag) | <i>I</i><br>(mag) | Telescope                 |
|-----------|-------------------|-------------------|-------------------|-----------------------|-------------------|---------------------------|
| 57462.384 | -                 | -                 | -                 | 16.896 ± 0.190        | -                 |                           |
| 57463.381 | 17.196 ± 0.160    | 16.691 ± 0.131    | 16.488 ± 0.165    | 16.553 ± 0.226        | 16.381 ± 0.124    | KAIT                      |
| 57464.338 | 16.843 ± 0.119    | 16.408 ± 0.080    | 16.180 ± 0.102    | 16.199 ± 0.103        | 16.079 ± 0.086    | KAIT                      |
| 57465.324 | 16.879 ± 0.120    | 16.192 ± 0.066    | 16.027 ± 0.070    | 15.967 ± 0.131        | 15.809 ± 0.106    | KAIT                      |
| 57466.310 | 16.726 ± 0.134    | 16.005 ± 0.057    | 15.852 ± 0.055    | 15.838 ± 0.105        | 15.661 ± 0.063    | KAIT                      |
| 57467.330 | 16.787 ± 0.253    | 15.890 ± 0.103    | 15.608 ± 0.098    | 15.767 ± 0.156        | 15.451 ± 0.128    | KAIT                      |
| 57470.385 | 16.762 ± 0.165    | 15.741 ± 0.071    | 15.376 ± 0.074    | 15.374 ± 0.061        | 15.165 ± 0.091    | KAIT                      |
| 57471.397 | 16.401 ± 0.176    | 15.589 ± 0.059    | 15.278 ± 0.053    | 15.288 ± 0.062        | 15.114 ± 0.056    | KAIT                      |
| 57472.397 | 16.358 ± 0.140    | 15.477 ± 0.061    | 15.202 ± 0.051    | 15.254 ± 0.065        | 15.031 ± 0.055    | KAIT                      |
| 57473.355 | 16.282 ± 0.114    | 15.467 ± 0.049    | 15.196 ± 0.049    | 15.206 ± 0.072        | 14.982 ± 0.055    | KAIT                      |
| 57474.383 | 16.106 ± 0.315    | 15.464 ± 0.083    | 15.107 ± 0.063    | 15.154 ± 0.075        | 14.882 ± 0.114    | KAIT                      |
| 57476.373 | 16.079 ± 0.131    | 15.398 ± 0.048    | 15.026 ± 0.049    | 15.067 ± 0.079        | 14.806 ± 0.052    | KAIT                      |
| 57477.367 | 16.274 ± 0.088    | 15.348 ± 0.042    | 15.048 ± 0.042    | 15.073 ± 0.046        | 14.787 ± 0.042    | KAIT                      |
| 57478.332 | 16.340 ± 0.082    | 15.376 ± 0.044    | 15.005 ± 0.042    | 15.055 ± 0.080        | 14.744 ± 0.040    | KAIT                      |
| 57479.395 | 16.290 ± 0.123    | 15.365 ± 0.054    | 14.989 ± 0.053    | 15.039 ± 0.089        | 14.750 ± 0.060    | KAIT                      |
| 57480.345 | 16.440 ± 0.087    | 15.422 ± 0.034    | 15.037 ± 0.038    | 15.062 ± 0.045        | 14.753 ± 0.056    | KAIT                      |
| 57481.338 | 16.487 ± 0.207    | 15.444 ± 0.070    | 15.102 ± 0.065    | 15.105 ± 0.073        | 14.713 ± 0.062    | KAIT                      |
| 57482.341 | 16.801 ± 0.142    | 15.527 ± 0.053    | 15.057 ± 0.045    | 15.132 ± 0.065        | 14.784 ± 0.049    | KAIT                      |
| 57485.358 | 17.453 ± 0.207    | 15.691 ± 0.115    | 15.237 ± 0.093    | 15.320 ± 0.090        | 15.039 ± 0.090    | KAIT                      |
| 57491.352 | 17.914 ± 0.243    | 16.282 ± 0.118    | 15.730 ± 0.119    | 15.744 ± 0.141        | 15.224 ± 0.116    | KAIT                      |
| 57492.352 | 17.765 ± 0.159    | 16.376 ± 0.103    | 15.776 ± 0.085    | 15.824 ± 0.137        | 15.262 ± 0.073    | KAIT                      |
| 57494.257 | 17.979 ± 0.169    | 16.484 ± 0.108    | 15.896 ± 0.111    | 15.941 ± 0.148        | 15.392 ± 0.125    | KAIT                      |
| 57495.299 | 18.142 ± 0.134    | 16.553 ± 0.069    | 15.914 ± 0.071    | 16.018 ± 0.095        | 15.427 ± 0.064    | KAIT                      |
| 57496.272 | 18.106 ± 0.131    | 16.603 ± 0.065    | 15.970 ± 0.063    | 16.048 ± 0.093        | 15.445 ± 0.058    | KAIT                      |
| 57497.268 | 18.194 ± 0.186    | 16.721 ± 0.086    | 15.966 ± 0.065    | 16.100 ± 0.084        | 15.492 ± 0.067    | KAIT                      |
| 57498.330 | 18.137 ± 0.145    | 16.646 ± 0.094    | 16.065 ± 0.087    | 16.129 ± 0.114        | 15.557 ± 0.079    | KAIT                      |
| 57499.317 | 18.147 ± 0.329    | 16.675 ± 0.149    | 16.111 ± 0.141    | 16.193 ± 0.230        | 15.555 ± 0.131    | KAIT                      |
| 57502.338 | 18.204 ± 0.277    | 16.935 ± 0.170    | 16.180 ± 0.204    | 16.201 ± 0.147        | 15.674 ± 0.095    | KAIT                      |
| 57504.271 | 18.340 ± 0.173    | 16.893 ± 0.111    | 16.291 ± 0.114    | 16.313 ± 0.165        | 15.738 ± 0.095    | KAIT                      |
| 57505.327 | -                 | -                 | -                 | 16.297 ± 0.148        | -                 | KAIT                      |
| 57507.265 | 18.362 ± 0.179    | 16.974 ± 0.109    | 16.372 ± 0.116    | 16.408 ± 0.184        | 15.803 ± 0.089    | KAIT                      |
| 57508.241 | 18.348 ± 0.248    | 16.993 ± 0.197    | 16.445 ± 0.210    | 16.408 ± 0.237        | 15.837 ± 0.163    | KAIT                      |
| 57509.285 | 18.414 ± 0.156    | 17.023 ± 0.110    | 16.401 ± 0.119    | 16.441 ± 0.181        | 15.825 ± 0.098    | KAIT                      |
| 57510.229 | -                 | -                 | -                 | 16.458 ± 0.172        | -                 | KAIT                      |
| 57511.236 | 18.498 ± 0.154    | 17.092 ± 0.121    | 16.484 ± 0.086    | 16.447 ± 0.178        | 15.848 ± 0.087    | KAIT                      |
| 57513.195 | 18.490 ± 0.417    | 17.150 ± 0.163    | 16.552 ± 0.134    | 16.517 ± 0.195        | 15.929 ± 0.112    | KAIT                      |
| 57517.272 | 18.501 ± 0.189    | 17.238 ± 0.104    | 16.619 ± 0.116    | 16.594 ± 0.221        | 16.001 ± 0.096    | KAIT                      |
| 57518.210 | 18.590 ± 0.151    | 17.221 ± 0.129    | 16.668 ± 0.114    | 16.591 ± 0.139        | 15.993 ± 0.094    | KAIT                      |
| 57519.223 | 18.514 ± 0.156    | 17.211 ± 0.094    | 16.671 ± 0.095    | 16.612 ± 0.127        | 16.043 ± 0.101    | KAIT                      |
| 57520.193 | 18.453 ± 0.167    | 17.284 ± 0.148    | 16.669 ± 0.099    | 16.651 ± 0.349        | 16.039 ± 0.102    | KAIT                      |
| 57521.203 | 18.651 ± 0.179    | 17.276 ± 0.126    | 16.737 ± 0.121    | 16.699 ± 0.119        | 16.057 ± 0.093    | KAIT                      |
| 57522.186 | 18.638 ± 0.215    | 17.359 ± 0.186    | 16.744 ± 0.190    | 16.727 ± 0.263        | 16.074 ± 0.155    | KAIT                      |
| 57523.259 | 18.510 ± 0.235    | 17.396 ± 0.194    | 16.697 ± 0.149    | 16.672 ± 0.322        | 16.029 ± 0.118    | KAIT                      |
| 57524.206 | 18.643 ± 0.147    | 17.346 ± 0.121    | 16.717 ± 0.116    | 16.753 ± 0.229        | 16.068 ± 0.102    | KAIT                      |
| 57525.193 | 18.675 ± 0.168    | 17.392 ± 0.090    | 16.802 ± 0.118    | 16.729 ± 0.134        | 16.117 ± 0.110    | KAIT                      |
| 57526.218 | 18.464 ± 0.205    | 17.358 ± 0.120    | 16.748 ± 0.113    | 16.739 ± 0.243        | 16.097 ± 0.101    | KAIT                      |
| 57527.200 | 18.490 ± 0.166    | 17.401 ± 0.092    | 16.824 ± 0.116    | 16.846 ± 0.201        | 16.115 ± 0.089    | KAIT                      |
| 57531.212 | 18.761 ± 0.175    | 17.450 ± 0.096    | 16.854 ± 0.102    | 16.832 ± 0.221        | 16.214 ± 0.114    | KAIT                      |
| 57533.227 | 18.663 ± 0.143    | 17.541 ± 0.109    | 16.914 ± 0.143    | 16.848 ± 0.249        | 16.209 ± 0.075    | KAIT                      |
| 57534.202 | 18.583 ± 0.130    | 17.519 ± 0.085    | 16.984 ± 0.133    | 16.933 ± 0.264        | 16.271 ± 0.102    | KAIT                      |
| 57535.215 | 18.683 ± 0.163    | 17.558 ± 0.110    | 16.998 ± 0.112    | 16.975 ± 0.277        | 16.269 ± 0.105    | KAIT                      |
| 57536.219 | 18.693 ± 0.177    | 17.587 ± 0.101    | 16.981 ± 0.103    | 16.958 ± 0.257        | 16.275 ± 0.076    | KAIT                      |
| 57537.232 | 18.818 ± 0.224    | 17.562 ± 0.098    | 17.001 ± 0.093    | 17.010 ± 0.270        | 16.257 ± 0.093    | KAIT                      |
| 57541.231 | 18.793 ± 0.151    | 17.682 ± 0.086    | 17.137 ± 0.117    | 16.981 ± 0.263        | 16.355 ± 0.097    | KAIT                      |
| 57552.211 | 18.943 ± 0.150    | 17.819 ± 0.124    | 17.316 ± 0.100    | 17.231 ± 0.070        | 16.525 ± 0.088    | KAIT                      |
| 57572.191 | 19.171 ± 0.331    | 18.126 ± 0.132    | 17.587 ± 0.117    | 17.422 ± 0.139        | 16.842 ± 0.118    | KAIT                      |
| 57574.190 | -                 | -                 | -                 | 17.403 ± 0.091        | -                 | KAIT                      |
| 57576.191 | -                 | -                 | -                 | 17.544 ± 0.519        | -                 | KAIT                      |
| 57471.326 | 16.267 ± 0.022    | 15.589 ± 0.015    | 15.274 ± 0.019    | -                     | 15.065 ± 0.027    | KAIT                      |
| 57484.382 | 16.823 ± 0.029    | 15.501 ± 0.034    | 15.213 ± 0.014    | -                     | 14.842 ± 0.022    | KAIT                      |
| 57498.264 | 17.822 ± 0.081    | 16.741 ± 0.057    | 16.069 ± 0.031    | -                     | 15.551 ± 0.035    | KAIT                      |
| 57511.285 | 18.314 ± 0.376    | 17.054 ± 0.046    | 16.397 ± 0.025    | -                     | 15.843 ± 0.616    | KAIT                      |
| 57535.248 | 18.563 ± 0.058    | 17.544 ± 0.035    | 16.948 ± 0.044    | -                     | 16.289 ± 0.072    | KAIT                      |
| 57541.241 | 18.555 ± 0.719    | 17.565 ± 0.070    | 17.014 ± 0.034    | -                     | 16.347 ± 0.028    | KAIT                      |
| 57546.216 | 18.816 ± 0.229    | 17.691 ± 0.070    | 17.139 ± 0.028    | -                     | 16.447 ± 0.099    | KAIT                      |
| 57587.185 | 19.431 ± 0.701    | 18.453 ± 0.309    | -                 | -                     | -                 | MNRAS 000, 000–000 (0000) |
